# Supplementary material for: Scraping the Shadows: Deep Learning Breakthroughs in Dark Web Intelligence
Source: arXiv:2504.02872 source file (2025-04-01)
Supplement: Supplementary file 1 [file appendix.tex]

% \section*{Appendix}

% \begin{table}[h!]
% \begin{tabular}{|ll|}
% \hline
% \multicolumn{1}{|l|}{\textbf{Entity}}      & \textbf{RegEx Pattern}                                                                    \\ \hline
% \multicolumn{2}{|c|}{\textbf{Agartha Item}}                                                                                            \\ \hline
% \multicolumn{1}{|l|}{market\_name}         & (\textbackslash w+)\textbackslash s+purchase                                              \\ \hline
% \multicolumn{1}{|l|}{product}              & (?:listings.*?)1listings\textbackslash s+(.+?)\textbackslash s+message                    \\ \hline
% \multicolumn{1}{|l|}{model}                & category\textbackslash s+(\textbackslash w+)                                              \\ \hline
% \multicolumn{1}{|l|}{quantity\_in\_stock}  & availability (\textbackslash d+)                                                          \\ \hline
% \multicolumn{1}{|l|}{product\_price}       & price (\textbackslash d+\textbackslash .\textbackslash d+)                                \\ \hline
% \multicolumn{1}{|l|}{product\_description} & listings (.+?) purchase                                                                   \\ \hline
% \multicolumn{1}{|l|}{product\_views}       & (\textbackslash d+)\textbackslash s+\textbackslash d+,\textbackslash d+\textbackslash s?€ \\ \hline
% \multicolumn{1}{|l|}{vendor\_name}         & vendor\textbackslash s+(\textbackslash w+)                                                \\ \hline
% \multicolumn{2}{|c|}{\textbf{Agartha Purchase}}                                                                                        \\ \hline
% \multicolumn{1}{|l|}{market\_name}         & (\textbackslash w+)\textbackslash s+purchase                                              \\ \hline
% \multicolumn{1}{|l|}{product}              & (?:purchase.*?)1purchase\textbackslash s+(.+?)\textbackslash s+category                   \\ \hline
% \multicolumn{1}{|l|}{model}                & category\textbackslash s+(\textbackslash w+)                                              \\ \hline
% \multicolumn{1}{|l|}{quantity\_in\_stock}  & availability (\textbackslash d+)                                                          \\ \hline
% \multicolumn{1}{|l|}{product\_price}       & (\textbackslash d+\textbackslash .\textbackslash d+)\textbackslash s+(usd|btc)            \\ \hline
% \multicolumn{1}{|l|}{product\_description} & listings (.+?) purchase                                                                   \\ \hline
% \multicolumn{1}{|l|}{product\_views}       & (\textbackslash d+)\textbackslash s+\textbackslash d+,\textbackslash d+\textbackslash s?€ \\ \hline
% \multicolumn{1}{|l|}{vendor\_name}         & vendor\textbackslash s+(\textbackslash w+)                                                \\ \hline
% \multicolumn{2}{|c|}{\textbf{Berlusconi}}                                                                                              \\ \hline
% \multicolumn{1}{|l|}{market\_name}         & \textbackslash berlusconi\textbackslash b                                                 \\ \hline
% \multicolumn{1}{|l|}{product} & $^(.+?)$\textbackslash s\d+(?:\textbackslash .\textbackslash d+)?\textbackslash s*eur \\ \hline
% \multicolumn{1}{|l|}{model}                & class\textbackslash s+(\textbackslash w+)                                                 \\ \hline
% \multicolumn{1}{|l|}{quantity\_in\_stock}  & (\textbackslash d+) s+in stock                                                            \\ \hline
% \multicolumn{1}{|l|}{product\_price}       & (\textbackslash d+(?:\textbackslash .\textbackslash d+)?)(?=\textbackslash s+eur)         \\ \hline
% \multicolumn{1}{|l|}{product\_description} & avis (.+?) modèle                                                                         \\ \hline
% \multicolumn{1}{|l|}{product\_views}       & (\textbackslash d+)\textbackslash s+\textbackslash d+,\textbackslash d+\textbackslash s?€ \\ \hline
% \multicolumn{1}{|l|}{vendor\_name}         & vendor\textbackslash s+(\textbackslash w+)                                                \\ \hline
% \multicolumn{2}{|c|}{\textbf{Cannahome}}                                                                                               \\ \hline
% \multicolumn{1}{|l|}{market\_name}         & (\textbackslash w+)\textbackslash s+purchase                                              \\ \hline
% \multicolumn{1}{|l|}{product}              & details (.+?) availability                                                                \\ \hline
% \multicolumn{1}{|l|}{model}                & category\textbackslash s+(\textbackslash w+)                                              \\ \hline
% \multicolumn{1}{|l|}{quantity\_in\_stock}  & availability (\textbackslash d+)                                                          \\ \hline
% \multicolumn{1}{|l|}{product\_price}       & escrow (\textbackslash d+.\textbackslash d+)                                              \\ \hline
% \multicolumn{1}{|l|}{product\_description} & avis (.+?) modèle                                                                         \\ \hline
% \multicolumn{1}{|l|}{product\_views}       & (\textbackslash w+)\textbackslash s+orders                                                \\ \hline
% \multicolumn{1}{|l|}{vendor\_name}         & vendor\textbackslash s+(\textbackslash w+)                                                \\ \hline
% \multicolumn{2}{|c|}{\textbf{Cocorico}}                                                                                                \\ \hline
% \multicolumn{1}{|l|}{market\_name}         & \textbackslash bcocorico\textbackslash s market\textbackslash b                           \\ \hline
% \multicolumn{1}{|l|}{product}              & recherche (.+?) description                                                               \\ \hline
% \multicolumn{1}{|l|}{model}                & modèle\textbackslash s+(.+?)\textbackslash s+disponibilité                                \\ \hline
% \multicolumn{1}{|l|}{quantity\_in\_stock}  & disponibilité :(\textbackslash d+)                                                        \\ \hline
% \multicolumn{1}{|l|}{product\_price}       & (\textbackslash d+, d+)\textbackslash s?€                                                 \\ \hline
% \multicolumn{1}{|l|}{product\_description} & avis (.+?) modèle                                                                         \\ \hline
% \multicolumn{1}{|l|}{product\_views}       & (\textbackslash d+)\textbackslash s+\textbackslash d+,\textbackslash d+\textbackslash s?€ \\ \hline
% \multicolumn{1}{|l|}{vendor\_name}         & (\textbackslash b\textbackslash w+\textbackslash b)\textbackslash s+rating                \\ \hline
% \multicolumn{2}{|c|}{\textbf{Dark Market}}                                                                                             \\ \hline
% \multicolumn{1}{|l|}{market\_name}         & (\textbackslash w+)\textbackslash s+purchase                                              \\ \hline
% \multicolumn{1}{|l|}{product}              & 1 (.+?) quality                                                                           \\ \hline
% \multicolumn{1}{|l|}{model}                & type\textbackslash s+(\textbackslash w+)                                                  \\ \hline
% \multicolumn{1}{|l|}{quantity\_in\_stock}  & leftsold (\textbackslash d+)                                                              \\ \hline
% \multicolumn{1}{|l|}{product\_price}       & offers (\textbackslash d+\textbackslash .+\textbackslash d+)                              \\ \hline
% \multicolumn{1}{|l|}{product\_description} & listings (.+?) quality                                                                    \\ \hline
% \multicolumn{1}{|l|}{product\_views}       & (\textbackslash d+)\textbackslash s+\textbackslash d+,\textbackslash d+\textbackslash s?€ \\ \hline
% \multicolumn{1}{|l|}{vendor\_name}         & information\textbackslash s+(\textbackslash w+)                                           \\ \hline
% \multicolumn{2}{|l|}{Silkroad}                                                                                                         \\ \hline
% \multicolumn{1}{|l|}{market\_name}         & \textbackslash bsilk\textbackslash s road\textbackslash b                                 \\ \hline
% \multicolumn{1}{|l|}{product}              & usd+(.+?)\textbackslash s+price                                                           \\ \hline
% \multicolumn{1}{|l|}{model}                & category+(.+?)\textbackslash s+stock                                                      \\ \hline
% \multicolumn{1}{|l|}{quantity\_in\_stock}  & remaining\textbackslash s*(\textbackslash d+)                                             \\ \hline
% \multicolumn{1}{|l|}{product\_price}       & price s*(\textbackslash d+)                                                               \\ \hline
% \multicolumn{1}{|l|}{product\_description} & avis (.+?) modèle                                                                         \\ \hline
% \multicolumn{1}{|l|}{product\_views}       & (\textbackslash d+)\textbackslash s+\textbackslash d+,\textbackslash d+\textbackslash s?€ \\ \hline
% \multicolumn{1}{|l|}{vendor\_name}         & listings\textbackslash s+(\textbackslash w+)                                              \\ \hline
% \end{tabular}
% \caption{Combined RegEx Patterns for Retrieving Entities from Various DNMs}
% \label{tab:combined-regex-patterns}
% \end{table}
